# Supplementary material for: Adversarial purification with Score-based generative models
Source: arXiv:2106.06041 source file (2021-06-11)
Supplement: Supplementary file 1 [file ChD_FullBlind.tex]

\section{Additional defense results}
\label{sec:additionaldef}
\subsection{Full defense results for preprocessor-blind attacks}
\label{sec:preprocessorblind}
\begin{table}[!htb]
\caption{\label{table:pbfull}Evaluation results for preprocessor-blind attacks without noise injection and deterministic step sizes, starting with $\alpha_1=0.08$ and $\alpha_L=8.0\times 10^{-4}$ with $L=10$. Threat model: $l_\infty$ $\epsilon$-ball with $\epsilon=8/255$, CIFAR-10 dataset.}
\centering
\begin{tabular}{lllllll}
\toprule
\multirow{2}{*}{Method} & \multicolumn{2}{c}{Accuracy (\%)} & \multicolumn{2}{c}{Network architecture} & \multicolumn{2}{c}{Attack configuration} \\
\cmidrule{2-3}\cmidrule{4-5}\cmidrule{6-7}
 & Natural & Robust & Purifier & Classifier & Attack method & Threat blindness\\
 \midrule
ADP & & & & & \\
\hspace{3mm}Naturally Trained & 91.89 & 81.84 & \gls{ncsn}v2 & WRN-28-10 & Classifier \gls{pgd} & Unseen\\
\hspace{3mm}Naturally Trained & 91.90 & 82.96 & \gls{ncsn}v2 & WRN-28-10 & Classifier BIM & Unseen\\
\hspace{3mm}AT ($\epsilon=4/255$) & 91.90 & 90.59 & \gls{ncsn}v2 & WRN-28-10 & Classifier \gls{pgd} &Seen \\
\hspace{3mm}AT ($\epsilon=4/255$) & 91.90 & 88.46 & \gls{ncsn}v2 & WRN-28-10 & Classifier BIM & Seen\\
\hspace{3mm}AT ($\epsilon=8/255$) & 91.39 & {92.36} & \gls{ncsn}v2 & WRN-28-10 & Classifier \gls{pgd} &Seen\\
\hspace{3mm}AT ($\epsilon=8/255$) & 91.39 & 92.18 & \gls{ncsn}v2 & WRN-28-10 & Classifier BIM & Seen\\
\hspace{3mm}AT ($\epsilon=16/255$) & 91.73 & 89.58 & \gls{ncsn}v2 & WRN-28-10 & Classifier \gls{pgd} & Seen\\
\hspace{3mm}AT ($\epsilon=16/255$) & 91.73 & 89.81 & \gls{ncsn}v2 & WRN-28-10 & Classifier BIM & Seen\\
\hspace{3mm}Natural ($\sigma=0.15$) & 89.60 & 82.98 & \gls{ncsn}v2 & WRN-28-10 & Classifier \gls{pgd} & Unseen \\
\midrule
\citep{hill2020stochastic} & 84.12 & 78.91 & IGEBM & WRN-28-10 & Classifier \gls{pgd}&Unseen\\
\citep{shi2021online} & 84.07 & 51.42 & Self-supervised & ResNet-18 & Classifier \gls{pgd} & Unseen \\
\citep{shi2021online} & 91.89 & 53.58 & Self-supervised & WRN-28-10 & Classifier \gls{pgd} & Unseen \\
\citep{song2018pixeldefend} & 90 & 70 & PixelCNN & ResNet-62 & Classifier \gls{pgd} & Seen \\
\bottomrule
\end{tabular}
\end{table}
In this section, we present the full list of defense results for preprocessor-blind attacks containing those purified with noise injection in~\cref{table:pbfull}.
\subsection{Full list of defense results for more datasets}
\label{sec:extensive}
\input{tables/extensive}
We present the full list of defense results for various datasets, including MNIST, FashionMNIST, and CIFAR-100 in~\cref{table:extensive}.
